# Supplementary material for: Transformation of quantum photonic circuit models by term rewriting
Source: arXiv:1206.1104 source file (2012-06-06)
Supplement: Supplementary file 1 [file SupplementaryInformation.pdf]

# Supplementary Data for

# Transformation of quantum photonic circuit models by term rewriting


Gopal Sarma, Ryan Hamerly, Nikolas Tezak, Dmitri S. Pavlichin, Hideo Mabuchi

Edward L. Ginzton Laboratory, Stanford University, Stanford, CA 94305, USA


*Listings 1-4 referenced in the main article text are included in this Supplementary Data file. Online access to a complete version of our quantum photonic circuit analysis software can be obtained by contacting the authors. Details of the nine-qubit QEC circuit model with propagation losses are included after the code listings.*

---

## Listing 1: Insertion of propagation losses

```
generateLosses[modelName_] := Module[{rules, N, Losses, LNames},
  (*Import connectivity map*)
  (*# of losses given by # of beam paths*)
  rules = modelName[connectListToRules];
  N = rules // Length;
  (*Define lossy components and names for symbolic expressions*)
  Losses = Table[StringJoin["Loss", "L", ToString[i], "]"], {i, 1, N}];
  LNames = Table[Subscript[
     StringJoin["L", ToString[i] / ToExpression, 1]], {i, 1, N}];
  (*Append components to original model*)
  AppendTo[modelName[ToSLH], Losses];
  (*Transform netlist to incorporate losses*)
  MapIndexed[
    (# /. (A_a_ → B_b_) →
        {A_a → LNames[[First[#2]]], LNames[[First[#2]]] → B_b}) &,
    rules
   ] // Flatten
 ]
```

# Listing 2: Netlist conversion to a Gough-James circuit expression

The circuit parsing algorithm described in the article is summarized by the following pseudocode:

```
Repeat
   Find connectivity score for all component pairs
   Find pair with highest score
   Combine the two components of the pair; get circuit with N-1 components
Until no connections left
```

```
ConnReduce::err = "Fatal error.  Circuit reduction halted.";
ConnReduce[R_Circuit] := Module[{ans = R, ans0 = R, error = False},
    While[If[MatchQ[ans, _Circuit] &&
      UnsameQ[ans[[2]], {}] && CheckCircuit[ans], True,
         If[UnsameQ[ans[[2]], {}], error = True;
      Message[ConnReduce::err]]; False],
         ans0 = ans;
         ans = ConnReduceStep[ans0]];
    If[error, ans0, ans]]
ConnReduceStep[R_Circuit] := Module[{i, iMax, scMax = 0, sc},
    For[i = 1, i <= Length[R[[2]]], i++,
         Which[ConnScore[R, R[[2, i]]] == 1, iMax = i; Break[],
              ConnScore[R, R[[2, i]]] > scMax,
    scMax = ConnScore[R, R[[2, i]]]; iMax = i]];
              ConnReduceStep[R, R[[2, iMax]]]]
ConnReduceStep[R_Circuit, Am_Subscript -> Bn_Subscript] := Module[
    {AB, ABSymb, R1 = R[[1]], R2 = R[[2]],
   R3 = R[[3]], A = Am[[1]], B = Bn[[1]], m = Am[[2]], n = Bn[[2]], subs},
    If[SameQ[A, B],
         (* Connecting the same element (feedback). *)
         AB = Feedback[A, m, n]; ABSymb = GetNewSymbol[A, R1];
         R1 = R1 /. {A -> ABSymb};
         R2 = Cases[R2, Except[Am -> Bn]];
         subs = {(Subscript[A, i_] -> β_) :>
       (Subscript[ABSymb, If[i < m, i, i - 1]] -> β),
                (α_ -> Subscript[B, j_]) :>
       (α -> Subscript[ABSymb, If[j < n, j, j - 1]])};
         R2 = (R2 /. subs) /. subs;
         R3 = Append[R3, ABSymb -> AB];
         Circuit[R1, R2, R3],
         (* Connecting two different elements. *)
         Module[{nA, nB, connA, connB, nConn, nTot},
              {nA, nB} = {CDim[A], CDim[B]} //. R3;
              {connA, connB} =
      Cases[R2, (Subscript[A, i_] -> Subscript[B, j_]) -> {i, j}]^T;
              nConn = Length[connA]; nTot = nA + nB - nConn;
```

```
    ABSymb = GetNewSymbol[GetSymbol[B] <> GetSymbol[A], R1];
          {AB, subs} = ConnReduceHelper[A,
      B, ABSymb, nA, nB, connA, connB];
          R1 = Append[Complement[R1, {A, B}], ABSymb];
          R2 = Cases[R2, Except[Subscript[A, _] -> Subscript[B, _]]];
          R2 = (R2 /. subs) /. subs;
          R3 = Append[R3, (ABSymb -> AB)];
          Circuit[R1, R2, R3]]]]
ConnReduceHelper[A_, B_, AB_, nA_, nB_, connA_, connB_] :=
    Module[
  {Δn, ΔnMax, nPadMax, subsMax, subsInMax, subsOutMax, errMax, err,
    nConn = Length[connA], nTot = nA + nB - Length[connA]},
    errMax = 10^10;
    For[Δn = -(nB - nConn), Δn <= nA - nConn, Δn++,
       Module[{nPadATop = Max[-Δn, 0],
     nPadBTop = Max[Δn, 0], nPadABottom, nPadBBottom,
          portsA, portsB, portsnotA, portsnotB,
     notConnA, notConnB, subs},
          nPadABottom = nTot - nA - nPadATop;
    nPadBBottom = nTot - nB - nPadBTop;
          portsA = Range[nPadATop + 1, nPadATop + nA];
    portsB = Range[nPadBTop + 1, nPadBTop + nB];
          portsnotA = Complement[Range[nTot], portsA];
    portsnotB = Complement[Range[nTot], portsB];
          notConnA = Complement[Range[nA], connA];
    notConnB = Complement[Range[nB], connB];
          subs = {Join[portsA[[connA]], portsA[[notConnA]], portsnotA],
             Join[portsB[[connB]], portsnotB, portsB[[notConnB]]]}ᵀ /.
             {{a : Except[_List], b : Except[_List]} :> (a -> b)};
          (*Print["Δn: ", Δn, ", A: ", portsA, ", B: ", portsB];
          Print["subs: ", subs];

    Print["err: ", err=Total[Abs[Range[nTot]-(Range[nTot]/.subs)]]];*)
          If[(err = Total[Abs[Range[nTot] - (Range[nTot] /. subs)]]) <
      errMax,
             errMax = err; ΔnMax = Δn; subsMax = subs;

     nPadMax = {nPadATop, nPadABottom, nPadBTop, nPadBBottom};
             subsInMax = Join[Table[(α_ -> Subscript[A, i]) →

        (α -> Subscript[AB, portsA[[i]]]), {i, nA}],
                                        Table[
       (α_ -> Subscript[B, notConnB[[i]]]) →
```

```
          (α -> Subscript[AB, portsnotA[[i]]]),
                                                  {i, nTot - nA}]];
              subsOutMax = Join[
                     Table[

        (Subscript[A, notConnA[[i]]] -> β_) →
                          (Subscript[AB, portsnotB[[i]]] -> β),
        {i, nTot - nB}
                     ],
                  Table[(Subscript[B, i] -> β_) ->
          (Subscript[AB, portsB[[i]]] -> β), {i, nB}]]]]];
    (*Print[subsInMax/.{α$->α}, subsOutMax/.{β$->β}];*)
    {SeriesProduct[
     Concatenation[CIdentity[nPadMax[[3]]], B, CIdentity[nPadMax[[4]]]],
    CPermutation[Range[nTot] /. subsMax],
     Concatenation[CIdentity[nPadMax[[1]]], A,
    CIdentity[nPadMax[[2]]]]], Join[subsInMax /. {α$ -> α},
     subsOutMax /. {β$ -> β}]}]
```

```
ConnReduce::err = "Fatal error.  Circuit reduction halted.";
ConnReduce[R_Circuit] := Module[{ans = R, ans0 = R, error = False},
    While[If[MatchQ[ans, _Circuit] &&
      UnsameQ[ans[[2]], {}] && CheckCircuit[ans], True,
        If[UnsameQ[ans[[2]], {}], error = True;
      Message[ConnReduce::err]]; False],
        ans0 = ans;
        ans = ConnReduceStep[ans0]];
    If[error, ans0, ans]]
ConnReduceStep[R_Circuit] := Module[{i, iMax, scMax = 0, sc},
    For[i = 1, i <= Length[R[[2]]], i++,
        Which[ConnScore[R, R[[2,i]]] == 1, iMax = i; Break[],
            ConnScore[R, R[[2,i]]] > scMax,
    scMax = ConnScore[R, R[[2,i]]]; iMax = i]];
            ConnReduceStep[R, R[[2,iMax]]]]
ConnReduceStep[R_Circuit, Am_Subscript -> Bn_Subscript] := Module[
    {AB, ABSymb, R1 = R[[1]], R2 = R[[2]],
   R3 = R[[3]], A = Am[[1]], B = Bn[[1]], m = Am[[2]], n = Bn[[2]], subs},
    If[SameQ[A, B],
        (* Connecting the same element (feedback). *)
        AB = Feedback[A, m, n]; ABSymb = GetNewSymbol[A, R1];
        R1 = R1 /. {A -> ABSymb};
        R2 = Cases[R2, Except[Am -> Bn]];
        subs = {(Subscript[A, i_] -> β_) :>
```

```
        (Subscript[ABSymb, If[i < m, i, i - 1]] -> β),
                  (α_ -> Subscript[B, j_]) :>
        (α -> Subscript[ABSymb, If[j < n, j, j - 1]]])};
        R2 = (R2 /. subs) /. subs;
        R3 = Append[R3, ABSymb -> AB];
        Circuit[R1, R2, R3],
        (* Connecting two different elements. *)
        Module[{nA, nB, connA, connB, nConn, nTot},
            {nA, nB} = {CDim[A], CDim[B]} //. R3;
            {connA, connB} =
      Cases[R2, (Subscript[A, i_] -> Subscript[B, j_]) -> {i, j}]ᵀ;
            nConn = Length[connA]; nTot = nA + nB - nConn;

     ABSymb = GetNewSymbol[GetSymbol[B] <> GetSymbol[A], R1];
            {AB, subs} = ConnReduceHelper[A,
       B, ABSymb, nA, nB, connA, connB];
            R1 = Append[Complement[R1, {A, B}], ABSymb];
            R2 = Cases[R2, Except[Subscript[A, _] -> Subscript[B, _]]];
            R2 = (R2 /. subs) /. subs;
            R3 = Append[R3, (ABSymb -> AB)];
            Circuit[R1, R2, R3]]]]
ConnReduceHelper[A_, B_, AB_, nA_, nB_, connA_, connB_] :=
     Module[
   {Δn, ΔnMax, nPadMax, subsMax, subsInMax, subsOutMax, errMax, err,
     nConn = Length[connA], nTot = nA + nB - Length[connA]},
     errMax = 10^10;
     For[Δn = -(nB - nConn), Δn <= nA - nConn, Δn++,
        Module[{nPadATop = Max[-Δn, 0],
      nPadBTop = Max[Δn, 0], nPadABottom, nPadBBottom,
            portsA, portsB, portsnotA, portsnotB,
      notConnA, notConnB, subs},
            nPadABottom = nTot - nA - nPadATop;
     nPadBBottom = nTot - nB - nPadBTop;
            portsA = Range[nPadATop + 1, nPadATop + nA];
     portsB = Range[nPadBTop + 1, nPadBTop + nB];
            portsnotA = Complement[Range[nTot], portsA];
     portsnotB = Complement[Range[nTot], portsB];
            notConnA = Complement[Range[nA], connA];
     notConnB = Complement[Range[nB], connB];
            subs = {Join[portsA[[connA]], portsA[[notConnA]], portsnotA],
                Join[portsB[[connB]], portsnotB, portsB[[notConnB]]]}ᵀ /.
                {{a : Except[_List], b : Except[_List]} :> (a -> b)};
            (*Print["Δn: ", Δn, ", A: ", portsA, ", B: ", portsB];
            Print["subs: ", subs];
```

```
    Print["err: ", err=Total[Abs[Range[nTot]-(Range[nTot]/.subs)]]];*)
          If[(err = Total[Abs[Range[nTot] - (Range[nTot] /. subs)]]) <
      errMax,
              errMax = err; ΔnMax = Δn; subsMax = subs;

     nPadMax = {nPadATop, nPadABottom, nPadBTop, nPadBBottom};
              subsInMax = Join[Table[(α_ -> Subscript[A, i]) →

        (α -> Subscript[AB, portsA[[i]]]), {i, nA}],
                                      Table[
       (α_ -> Subscript[B, notConnB[[i]]]) →

        (α -> Subscript[AB, portsnotA[[i]]]),
                                                        {i, nTot - nA}]];
              subsOutMax = Join[
                        Table[

       (Subscript[A, notConnA[[i]]] -> β_) →
                       (Subscript[AB, portsnotB[[i]]] -> β),
       {i, nTot - nB}
                        ],
                  Table[(Subscript[B, i] -> β_) ->
        (Subscript[AB, portsB[[i]]] -> β), {i, nB}]]]]];
    (*Print[subsInMax/.{α$->α}, subsOutMax/.{β$->β}];*)
    {SeriesProduct[
    Concatenation[CIdentity[nPadMax[[3]]], B, CIdentity[nPadMax[[4]]]],
    CPermutation[Range[nTot] /. subsMax],
    Concatenation[CIdentity[nPadMax[[1]]], A,
    CIdentity[nPadMax[[2]]]]], Join[subsInMax /. {α$ -> α},
    subsOutMax /. {β$ -> β}]}]
```

```
ConnReduce::err = "Fatal error.  Circuit reduction halted.";
ConnReduce[R_Circuit] := Module[{ans = R, ans0 = R, error = False},
    While[If[MatchQ[ans, _Circuit] &&
      UnsameQ[ans[[2]], {}] && CheckCircuit[ans], True,
         If[UnsameQ[ans[[2]], {}], error = True;
      Message[ConnReduce::err]]; False],
         ans0 = ans;
         ans = ConnReduceStep[ans0]];
    If[error, ans0, ans]]
ConnReduceStep[R_Circuit] := Module[{i, iMax, scMax = 0, sc},
    For[i = 1, i <= Length[R[[2]]], i++,
         Which[ConnScore[R, R[[2,i]]] == 1, iMax = i; Break[],
```

```
            ConnScore[R, R[[2,i]]] > scMax,
    scMax = ConnScore[R, R[[2,i]]]; iMax = i]];
            ConnReduceStep[R, R[[2,iMax]]]]
ConnReduceStep[R_Circuit, Am_Subscript -> Bn_Subscript] := Module[
    {AB, ABSymb, R1 = R[[1]], R2 = R[[2]],
   R3 = R[[3]], A = Am[[1]], B = Bn[[1]], m = Am[[2]], n = Bn[[2]], subs},
    If[SameQ[A, B],
        (* Connecting the same element (feedback). *)
        AB = Feedback[A, m, n]; ABSymb = GetNewSymbol[A, R1];
        R1 = R1 /. {A -> ABSymb};
        R2 = Cases[R2, Except[Am -> Bn]];
        subs = {(Subscript[A, i_] -> β_) :>
      (Subscript[ABSymb, If[i < m, i, i - 1]] -> β),
                (α_ -> Subscript[B, j_]) :>
      (α -> Subscript[ABSymb, If[j < n, j, j - 1]])};
        R2 = (R2 /. subs) /. subs;
        R3 = Append[R3, ABSymb -> AB];
        Circuit[R1, R2, R3],
        (* Connecting two different elements. *)
        Module[{nA, nB, connA, connB, nConn, nTot},
            {nA, nB} = {CDim[A], CDim[B]} //. R3;
            {connA, connB} =
      Cases[R2, (Subscript[A, i_] -> Subscript[B, j_]) -> {i, j}]ᵀ;
            nConn = Length[connA]; nTot = nA + nB - nConn;

    ABSymb = GetNewSymbol[GetSymbol[B] <> GetSymbol[A], R1];
            {AB, subs} = ConnReduceHelper[A,
     B, ABSymb, nA, nB, connA, connB];
            R1 = Append[Complement[R1, {A, B}], ABSymb];
            R2 = Cases[R2, Except[Subscript[A, _] -> Subscript[B, _]]];
            R2 = (R2 /. subs) /. subs;
            R3 = Append[R3, (ABSymb -> AB)];
            Circuit[R1, R2, R3]]]]
ConnReduceHelper[A_, B_, AB_, nA_, nB_, connA_, connB_] :=
    Module[
   {Δn, ΔnMax, nPadMax, subsMax, subsInMax, subsOutMax, errMax, err,
    nConn = Length[connA], nTot = nA + nB - Length[connA]},
    errMax = 10^10;
    For[Δn = -(nB - nConn), Δn <= nA - nConn, Δn++,
        Module[{nPadATop = Max[-Δn, 0],
      nPadBTop = Max[Δn, 0], nPadABottom, nPadBBottom,
            portsA, portsB, portsnotA, portsnotB,
      notConnA, notConnB, subs},
            nPadABottom = nTot - nA - nPadATop;
```

```
nPadBBottom = nTot - nB - nPadBTop;
        portsA = Range[nPadATop + 1, nPadATop + nA];
portsB = Range[nPadBTop + 1, nPadBTop + nB];
        portsnotA = Complement[Range[nTot], portsA];
portsnotB = Complement[Range[nTot], portsB];
        notConnA = Complement[Range[nA], connA];
notConnB = Complement[Range[nB], connB];
        subs = {Join[portsA⟦connA⟧, portsA⟦notConnA⟧, portsnotA],
            Join[portsB⟦connB⟧, portsnotB, portsB⟦notConnB⟧]}ᵀ /.
            {{a : Except[_List], b : Except[_List]} :> (a -> b)};
        (*Print["Δn: ", Δn, ", A: ", portsA, ", B: ", portsB];
        Print["subs: ", subs];

Print["err: ", err=Total[Abs[Range[nTot]-(Range[nTot]/.subs)]]];*)
        If[(err = Total[Abs[Range[nTot] - (Range[nTot] /. subs)]]) <
  errMax,
            errMax = err; ΔnMax = Δn; subsMax = subs;

 nPadMax = {nPadATop, nPadABottom, nPadBTop, nPadBBottom};
            subsInMax = Join[Table[(α_ -> Subscript[A, i]) →

      (α -> Subscript[AB, portsA[[i]]]), {i, nA}],
                                  Table[
     (α_ -> Subscript[B, notConnB[[i]]]) →

      (α -> Subscript[AB, portsnotA[[i]]]),
                                                        {i, nTot - nA}]];
            subsOutMax = Join[
                    Table[

     (Subscript[A, notConnA[[i]]] -> β_) →
                          (Subscript[AB, portsnotB[[i]]] -> β),
     {i, nTot - nB}
                    ],
                Table[(Subscript[B, i] -> β_) ->
      (Subscript[AB, portsB[[i]]] -> β), {i, nB}]]]];
(*Print[subsInMax/.{α$->α}, subsOutMax/.{β$->β}];*)
{SeriesProduct[
Concatenation[CIdentity[nPadMax⟦3⟧], B, CIdentity[nPadMax⟦4⟧]],
CPermutation[Range[nTot] /. subsMax],
Concatenation[CIdentity[nPadMax⟦1⟧], A,
CIdentity[nPadMax⟦2⟧]]], Join[subsInMax /. {α$ -> α},
subsOutMax /. {β$ -> β}]}]
```

# Listing 3: Algebraic reduction to an overall (S,L,H) model

After the netlist has been transformed to a Gough-James circuit expression, component (**S, L,** H) parameters are combined according to series and concatenation-type products to obtain an overall (**S, L,** H) model for the entire circuit. Note that the parser we have described in the previous section is a completely general algorithm for transforming an arbitrary netlist for a system model into an algebraic expression of series and concatenation-type expressions. We first apply a series of transformations that replace the component symbols with their corresponding (**S, L,** H) representations.

- **Network Component Definitions**

```
BeamSplitter[x_] := Module[{},
CDim[x] = 2;
x[SLH] = {( 1/√2   1/√2
           -1/√2   1/√2 ), (0
                            0), 0}
];
```

```
Loss[x_] := Module[{},
CDim[x] = 2;
x[SLH] = {( Cos[θ/2]   Sin[θ/2]
           -Sin[θ/2]   Cos[θ/2] ), (0
                                    0), 0}
];
```

```
CoherentField[x_, amp_] := Module[{},
CDim[x] = 1;
x[SLH] = {(1), (amp), 0}
];
```

```
RelayPi[x_, y_] := Module[{},
CDim[x] = 2;
x[SLH] = {( Πg^y   -Πh^y
           -Πh^y    Πg^y ), (0
                            0), 0}
];
```

```
RelaySigma[x_, y_] := Module[{},
CDim[x] = 2;
x[SLH] = {( Π_g^y     -σ_{h,g}^y
           -σ_{g,h}^y    Π_h^y  ), (0
                                    0), 0}
];
```

```
Phase[x_] := Module[{},
CDim[x] = 1;
x[SLH] = {(ⅇ^{ⅈ ϕ}), (0), 0}
];
```

```
SingleCavity[x_, y_, z_] := Module[{},
CDim[x] = 1;
Which[SameQ[y, Ramang],
x[SLH] = {(1), (√γ σ_{g,r}^z), (Δ Π_r^z)/2},
SameQ[y, Ramanh],
x[SLH] = {(1), (√γ σ_{h,r}^z), (Δ Π_r^z)/2},
SameQ[y, Zprobe],
x[SLH] = {(Z^z), (0), 0},
SameQ[y, Xprobe],
x[SLH] = {(X^z), (0), 0}
]
];
```

```
cIdentity[n_] := Module[{},
CIdentity[n][SLH] =
    {IdentityMatrix[n], {ConstantArray[0, n]} // Transpose, 0}
];
```

```
cPermutation[c_List] := Module[{dim},
dim = Length[c];
CPermutation[c][SLH] = {Permute[IdentityMatrix[dim], c] // Transpose,
      {ConstantArray[0, dim]} // Transpose, 0}
];
```

## ■ Series and Concatenation Products

Note that until a proper (**S, L,** H) representation is given for each of the network components, the algebraic rules implementing the series $\triangleleft$ and concatenation $\oplus$ products simply remain unevaluated, which allows us to manipulate the network expression at a purely symbolic level before conversion to (**S, L,** H) form.

```
toArray[M_] := Module[{}, If[MatrixQ[M], M, List[List[M]]]]
```

```
seriesProduct1[{S1_, L1_, H1_}, {S2_, L2_, H2_}] :=
 Module[{S1p, L1p, S2p, L2p, H3, H4},
H3 = FunctionExpand[Im[Expand[ConjugateTranspose[toArray[L1]].
        toArray[S1].toArray[L2]]]] /. Im -> IM;
H4 = H3 /. IM[x_] :> ComplexExpand[Im[x], Level[x, 1],
      TargetFunctions -> Conjugate];
{toArray[S1].toArray[S2], toArray[S1].toArray[L2] + toArray[L1],
   H1 + H2 + H4}
]
```

```
seriesProduct[{S1_, L1_, H1_}, y__] := Module[{},
Fold[seriesProduct1, {S1, L1, H1}, {y}]
]
```

```
Clear[concatenationProduct, concatenationProduct1];
concatenationProduct1[{S1_, L1_, H1_}, {S2_, L2_, H2_}] := Module[{},
{ArrayFlatten[({{S1, 0}, {0, S2}})],
   ArrayFlatten[({{L1}, {L2}})], H1 + H2}
]
```

```
concatenationProduct[{S1_, L1_, H1_}, y__] := Module[{},
Fold[concatenationProduct1, {S1, L1, H1}, {y}]
]
```

## Rules and patterns for operator-valued SLH models

The (**S, L,** H) models themselves are symbolic expression consisting of quantum mechanical operators. In the term-rewriting paradigm, we implement the necessary symbolic transformations, in this case with *global* rather than the *local* rules that were defined previously. The key distinction is that global rules are applied to any instance of the corresponding symbols in a given session, whereas application of local rules is strictly specified by the user---this allows for expressions describing multiple levels of abstraction to be modeled and analyzed in a single setting. The following global rules are sufficient for the analysis of the quantum error correcting circuits described in this paper:

$$\left(\sigma_{g\_,h\_}{}^{Q\_}\right)^{\dagger} := \sigma_{h,g}{}^{Q};$$
$$\left(\Pi_{g\_}{}^{Q\_}\right)^{\dagger} := \Pi_{g}{}^{Q};$$
$$\left(\Pi_{g\_}{}^{Q\_}\right)^{2} := \Pi_{g}{}^{Q};$$
$$\Pi_{g\_}{}^{Q\_}\,\Pi_{h\_}{}^{Q\_}\ /;\ (g\ =!=\ h)\ :=\ \Pi_{g}{}^{Q}\,\delta_{g,h};$$
$$\Pi_{g\_}{}^{R1\_|R2\_} + \Pi_{h\_}{}^{R1\_|R2\_}\ /;\ (g\ ===\ h)\ :=\ 1;$$

# Listing 4: Model reduction using a QSDE limit theorem

Our analyses of the autonomous QEC memory circuits rely on a limit theorem for quantum stochastic differential equations to produce computationally tractable models for the overall network. This formalism can be viewed in two ways---as a technique for reducing the dimensionality of quantum photonic circuit models, and as a tool for moving to a level of abstraction in which the relevant network dynamics are transparently represented in analytic expressions.

The computation of reduced (limit) QEC circuit models can be automated using simple rewrite rules:

```
σg_,r^Q1_ σr,h_^Q2_ /; (UnsameQ[g, h] && SameQ[Q1, Q2]) → σg,h^Q1,
σg_,r^Q1_ σr,h_^Q2_ /; (SameQ[g, h] && SameQ[Q1, Q2]) → Πg^Q1,
σg_,r^Q1_ σr,h_^Q2_ /; UnsameQ[Q1, Q2] → 0
```

These rules form the heart of a simple algorithm for deriving reduced models for the QEC circuits.

```
AdiabaticElimination[pH_] := Module[{Lβ, dk, Lγ, S0dL0, A1, A2},
  (*Subcomponent for adiabatic elimination with large-
   field displacement*)
  Lβ = L /. γ → 0;
  dk = Simplify[ConjugateTranspose[S].Lβ] /. β → kβ;
  Lγ = L /. β → 0;
  S0dL0 = Simplify[ConjugateTranspose[S].Lγ];
  H1kt =
   -FunctionExpand[Im[Expand[Transpose[dk†].S0dL0]]] + (H /. β → kβ);
  (*Compue Hamiltonian from displaced subcomponent*)
  A1 = (Coefficient[pH, kβs] // Flatten) /. Plus → List // Transpose;
  A2 = (Coefficient[pH, kβ] // Flatten) /. Plus → List // Transpose;
  reducedHamiltonianAsList = Outer[Times, A1, A2] /. {
      σg_,r^Q1_ σr,h_^Q2_ /; (UnsameQ[g, h] && SameQ[Q1, Q2]) → σg,h^Q1,
      σg_,r^Q1_ σr,h_^Q2_ /; (SameQ[g, h] && SameQ[Q1, Q2]) → Πg^Q1,
      σg_,r^Q1_ σr,h_^Q2_ /; UnsameQ[Q1, Q2] → 0
     } // Flatten;
  reducedHamiltonian = reducedHamiltonianAsList /. List → Plus

 ]
```

# Gough-James expression for lossy nine-qubit QEC circuit

After parsing the netlist generated by the Modelica system designer we arrive at the following Gough-James expression. Here and in the following sections we only give the network model and corresponding Hamiltonian and coupling terms for the Z-probe and Z-feedback sub-circuits. The X-sub-circuits can be formed by appropriately permuting the qubit and relay indices and making the operator substitutions Z ↔X.

$$\begin{gathered}
(((((\mathrm{Q1} \oplus \mathcal{I}_1 \lhd \mathrm{L7}) \oplus \mathcal{I}_2 \lhd \mathcal{P}_{\{2,1,3,4\}} \lhd \mathcal{I}_1 \oplus (\mathcal{I}_1 \oplus (\mathrm{Q2} \oplus \mathcal{I}_1 \lhd \mathrm{L6}) \lhd \mathrm{B2} \oplus \mathcal{I}_1)) \oplus \mathcal{I}_3 \lhd \mathcal{P}_{\{1,2,4,5,6,3,7\}} \lhd \\
\mathcal{I}_3 \oplus (\mathcal{I}_2 \oplus \mathrm{L5} \lhd ((\mathrm{Q3} \lhd \mathrm{U1}) \oplus \mathcal{I}_2 \lhd \mathrm{L4} \oplus \mathcal{I}_1 \lhd \mathcal{P}_{\{2,1,3\}} \lhd \mathcal{I}_1 \oplus \mathrm{B1}) \oplus \mathcal{I}_1)) \oplus \mathcal{I}_1 \lhd \\
\mathcal{P}_{\{1,2,3,4,5,7,6,8\}} \lhd \mathcal{I}_6 \oplus (\mathrm{L2} \lhd \mathrm{W2} \oplus \mathcal{I}_1)) \oplus \mathcal{I}_2 \lhd \mathcal{P}_{\{1,2,3,4,6,7,8,5,9,10\}} \lhd \\
\mathcal{I}_7 \oplus ((\mathrm{L3} \lhd \mathrm{R1} \oplus \mathcal{I}_1) \oplus \mathcal{I}_1 \lhd \mathcal{P}_{\{2,1,3\}} \lhd \mathcal{I}_1 \oplus \mathrm{L1} \lhd \mathcal{I}_1 \oplus \mathrm{W1} \oplus \mathcal{I}_1)) \oplus \\
(((\mathrm{q2} \oplus \mathcal{I}_1 \lhd \mathrm{L14}) \oplus \mathcal{I}_6 \lhd \mathcal{P}_{\{2,1,3,4,5,6,7,8\}} \lhd \\
\mathcal{I}_1 \oplus (((\mathcal{I}_1 \oplus (\mathrm{q3} \oplus \mathcal{I}_1 \lhd \mathrm{L13}) \lhd \mathrm{B4} \oplus \mathcal{I}_1) \oplus \mathcal{I}_1 \lhd \mathcal{P}_{\{1,3,2,4\}} \lhd \mathcal{I}_2 \oplus \mathrm{L12}) \oplus \mathcal{I}_3 \lhd \mathcal{P}_{\{1,2,4,5,6,3,7\}} \lhd \\
\mathcal{I}_3 \oplus ((\mathrm{q1} \oplus \mathcal{I}_1 \lhd \mathrm{L11}) \oplus \mathcal{I}_2 \lhd \mathcal{P}_{\{2,1,3,4\}} \lhd \mathcal{I}_1 \oplus (\mathrm{B3} \oplus \mathcal{I}_1 \lhd \mathcal{I}_1 \oplus \mathrm{L8})))) \oplus \mathcal{I}_2 \lhd \\
\mathcal{P}_{\{1,2,3,4,5,7,8,6,9,10\}} \lhd \mathcal{I}_5 \oplus \mathrm{W4} \oplus \mathcal{I}_1 \oplus (\mathrm{L10} \oplus \mathcal{I}_1 \lhd \mathcal{P}_{\{2,1,3\}} \lhd \mathcal{I}_1 \oplus (\mathrm{R2} \oplus \mathcal{I}_1 \lhd \mathrm{L9} \lhd \mathrm{W3} \oplus \mathcal{I}_1))) \oplus \\
((((\mathcal{I}_1 \oplus (\mathrm{R1} \oplus \mathcal{I}_1 \lhd \mathcal{I}_1 \oplus \mathrm{L16}) \lhd \mathcal{P}_{\{2,1,3,4\}} \lhd \mathrm{L15} \oplus \mathcal{I}_2) \oplus \mathcal{I}_1 \lhd \mathcal{P}_{\{2,1,3,5,4\}} \lhd \\
\mathcal{I}_1 \oplus ((\mathrm{B2} \lhd \mathcal{I}_1 \oplus \mathrm{U2}) \oplus \mathcal{I}_1 \lhd \mathcal{I}_1 \oplus \mathrm{L13} \lhd \mathcal{I}_1 \oplus \mathrm{W2} \oplus \mathcal{I}_1) \oplus \mathcal{I}_1) \oplus \mathcal{I}_4 \lhd \mathcal{P}_{\{1,3,4,5,2,6,7,8,9\}} \lhd \\
\mathcal{I}_4 \oplus (((\mathrm{U1} \oplus \mathcal{I}_1 \lhd \mathrm{L9} \lhd \mathrm{Q1} \oplus \mathcal{I}_1) \oplus \mathcal{I}_1 \lhd \mathcal{P}_{\{2,1,3\}} \lhd \mathcal{I}_1 \oplus \mathrm{L8}) \oplus \mathcal{I}_2 \lhd \mathcal{P}_{\{1,3,2,4,5\}} \lhd \\
\mathcal{I}_2 \oplus ((\mathrm{Q4} \oplus \mathcal{I}_1 \lhd \mathrm{L7} \lhd (\mathrm{Q7} \lhd \mathrm{U}) \oplus \mathcal{I}_1) \oplus \mathcal{I}_1 \lhd \mathcal{P}_{\{2,1,3\}} \lhd \mathcal{I}_1 \oplus \mathrm{L5}))) \oplus \\
\mathcal{I}_{12} \lhd \mathcal{P}_{\{1,2,3,4,5,6,7,9,10,11,12,13,14,15,16,17,8,18,19,20,21\}} \lhd \\
\mathcal{I}_8 \oplus ((\mathcal{I}_1 \oplus ((\mathcal{I}_1 \oplus (\mathrm{R2} \oplus \mathcal{I}_1 \lhd \mathcal{I}_1 \oplus \mathrm{L18}) \lhd \mathcal{P}_{\{2,1,3,4\}} \lhd (\mathrm{L17} \oplus \mathcal{I}_1 \lhd \mathcal{P}_{\{2,1,3\}} \lhd \mathcal{I}_1 \oplus \mathrm{B3}) \oplus \mathcal{I}_1) \oplus \mathcal{I}_1 \lhd \\
\mathcal{P}_{\{1,2,4,3,5\}} \lhd \mathcal{I}_3 \oplus (\mathrm{U3} \oplus \mathcal{I}_1 \lhd \mathrm{L14} \lhd \mathrm{W3} \oplus \mathcal{I}_1)) \lhd \mathcal{P}_{\{3,1,2,4,5,6\}} \lhd \\
(\mathrm{U4} \oplus \mathcal{I}_1 \lhd \mathrm{L12} \lhd \mathrm{Q3} \oplus \mathcal{I}_1) \oplus \mathcal{I}_4) \oplus \mathcal{I}_7 \lhd \mathcal{P}_{\{2,3,4,5,6,1,7,8,9,10,11,12,13\}} \lhd \\
\mathcal{I}_5 \oplus ((((\mathrm{L11} \lhd \mathrm{Q6} \oplus \mathcal{I}_1) \oplus \mathcal{I}_1 \lhd \mathcal{P}_{\{2,1,3\}} \lhd \mathcal{I}_1 \oplus \mathrm{L10}) \oplus \mathcal{I}_2 \lhd \mathcal{P}_{\{1,3,4,2,5\}} \lhd \\
\mathcal{I}_2 \oplus (\mathcal{I}_1 \oplus (\mathrm{Q9} \oplus \mathcal{I}_1 \lhd \mathrm{L6}) \lhd (\mathrm{B1} \lhd \mathrm{Q8} \oplus \mathcal{I}_1) \oplus \mathcal{I}_1)) \oplus \mathcal{I}_3 \lhd \\
\mathcal{P}_{\{1,2,4,5,3,6,7,8\}} \lhd \mathcal{I}_4 \oplus (((\mathrm{L3} \lhd \mathrm{Q5} \oplus \mathcal{I}_1) \oplus \mathcal{I}_1 \lhd \mathcal{P}_{\{2,1,3\}} \lhd \mathcal{I}_1 \oplus \mathrm{L19}) \oplus \mathcal{I}_1 \lhd \\
\mathcal{P}_{\{1,3,2,4\}} \lhd \mathcal{I}_2 \oplus (\mathrm{Q2} \oplus \mathcal{I}_1 \lhd \mathrm{L1} \lhd \mathrm{W1} \oplus \mathcal{I}_1)))))
\end{gathered}$$

# Hamiltonian and coupling terms for lossy nine-qubit QEC circuit

- **Hamiltonian**

$$\begin{gathered}
\frac{1}{4}\,\Omega\left(\left(X^{Q2}\left(-1+Z^{R1}\right)+\sqrt{2}\,X^{Q3}\left(1+Z^{R1}\right)\right)\left(-1+Z^{R2}\right)-\sqrt{2}\,X^{Q1}\left(-1+Z^{R1}\right)\left(1+Z^{R2}\right)\right)+ \\
\theta^2\left(\frac{\Omega\,X^{Q1}\left(-12+17\,Z^{R1}-17\,Z^{R2}+22\,Z^{R1}\,Z^{R2}\right)}{32\sqrt{2}}-\frac{\Omega\,X^{Q3}\left(-12-17\,Z^{R1}+17\,Z^{R2}+22\,Z^{R1}\,Z^{R2}\right)}{32\sqrt{2}}+\right. \\
\left.\frac{1}{64}\left(-14\,\Omega\,X^{Q2}+19\,\Omega\,X^{Q2}\,Z^{R1}+19\,\Omega\,X^{Q2}\,Z^{R2}-24\,\Omega\,X^{Q2}\,Z^{R1}\,Z^{R2}\right)\right)
\end{gathered}$$

- **Coupling terms**

$$\begin{pmatrix}
\frac{\alpha\,\text{Cos}\left[\frac{\theta}{2}\right]\,\text{Sin}\left[\frac{\theta}{2}\right]}{\sqrt{2}} - \frac{\alpha\,\text{Cos}\left[\frac{\theta}{2}\right]^7\,\text{Sin}\left[\frac{\theta}{2}\right]\,Z^{Q1}\,Z^{Q2}\,Z^{Q4}\,Z^{Q5}\,Z^{Q7}\,Z^{Q8}}{\sqrt{2}} \\
-\frac{\alpha\,\text{Cos}\left[\frac{\theta}{2}\right]^2\,\Pi_g{}^{R1}}{\sqrt{2}} + \frac{\alpha\,\text{Cos}\left[\frac{\theta}{2}\right]^2\,\sigma_{h,g}{}^{R1}}{\sqrt{2}} + \alpha\,\text{Cos}\left[\frac{\theta}{2}\right]^7\,Z^{Q1}\,Z^{Q2}\,Z^{Q4}\,Z^{Q5}\,Z^{Q7}\,Z^{Q8}\left(\frac{\text{Cos}\left[\frac{\theta}{2}\right]\,\Pi_g{}^{R1}}{\sqrt{2}} + \frac{\text{Cos}\left[\frac{\theta}{2}\right]\,\sigma_{h,g}{}^{R1}}{\sqrt{2}}\right) \\
-\frac{\alpha\,\text{Cos}\left[\frac{\theta}{2}\right]^2\,\Pi_h{}^{R1}}{\sqrt{2}} + \frac{\alpha\,\text{Cos}\left[\frac{\theta}{2}\right]^2\,\sigma_{g,h}{}^{R1}}{\sqrt{2}} + \alpha\,\text{Cos}\left[\frac{\theta}{2}\right]^7\,Z^{Q1}\,Z^{Q2}\,Z^{Q4}\,Z^{Q5}\,Z^{Q7}\,Z^{Q8}\left(-\frac{\text{Cos}\left[\frac{\theta}{2}\right]\,\Pi_h{}^{R1}}{\sqrt{2}} - \frac{\text{Cos}\left[\frac{\theta}{2}\right]\,\sigma_{g,h}{}^{R1}}{\sqrt{2}}\right) \\
\frac{\alpha\,\text{Cos}\left[\frac{\theta}{2}\right]\,\text{Sin}\left[\frac{\theta}{2}\right]}{\sqrt{2}} + \frac{\alpha\,\text{Cos}\left[\frac{\theta}{2}\right]^7\,\text{Sin}\left[\frac{\theta}{2}\right]\,Z^{Q1}\,Z^{Q2}\,Z^{Q4}\,Z^{Q5}\,Z^{Q7}\,Z^{Q8}}{\sqrt{2}} \\
-\alpha\,\text{Sin}\left[\frac{\theta}{2}\right] \\
\alpha\,\text{Cos}\left[\frac{\theta}{2}\right]^6\,\text{Sin}\left[\frac{\theta}{2}\right]\,Z^{Q1}\,Z^{Q2}\,Z^{Q4}\,Z^{Q5}\,Z^{Q7}\,Z^{Q8} \\
\alpha\,\text{Cos}\left[\frac{\theta}{2}\right]^5\,\text{Sin}\left[\frac{\theta}{2}\right]\,Z^{Q2}\,Z^{Q4}\,Z^{Q5}\,Z^{Q7}\,Z^{Q8} \\
\alpha\,\text{Cos}\left[\frac{\theta}{2}\right]^4\,\text{Sin}\left[\frac{\theta}{2}\right]\,Z^{Q2}\,Z^{Q5}\,Z^{Q7}\,Z^{Q8} \\
-\alpha\,\text{Cos}\left[\frac{\theta}{2}\right]^3\,\text{Sin}\left[\frac{\theta}{2}\right]\,Z^{Q2}\,Z^{Q5}\,Z^{Q8} \\
\alpha\,\text{Cos}\left[\frac{\theta}{2}\right]^6\,\text{Sin}\left[\frac{\theta}{2}\right]\,Z^{Q2}\,Z^{Q3}\,Z^{Q5}\,Z^{Q6}\,Z^{Q8}\,Z^{Q9} \\
\frac{\alpha\,\text{Cos}\left[\frac{\theta}{2}\right]\,\text{Sin}\left[\frac{\theta}{2}\right]}{\sqrt{2}} - \frac{\alpha\,\text{Cos}\left[\frac{\theta}{2}\right]^7\,\text{Sin}\left[\frac{\theta}{2}\right]\,Z^{Q2}\,Z^{Q3}\,Z^{Q5}\,Z^{Q6}\,Z^{Q8}\,Z^{Q9}}{\sqrt{2}} \\
-\alpha\,\text{Cos}\left[\frac{\theta}{2}\right]\left(\frac{\text{Cos}\left[\frac{\theta}{2}\right]\,\Pi_g{}^{R2}}{\sqrt{2}} - \frac{\text{Cos}\left[\frac{\theta}{2}\right]\,\sigma_{h,g}{}^{R2}}{\sqrt{2}}\right) + \alpha\,\text{Cos}\left[\frac{\theta}{2}\right]^7\,Z^{Q2}\,Z^{Q3}\,Z^{Q5}\,Z^{Q6}\,Z^{Q8}\,Z^{Q9}\left(\frac{\text{Cos}\left[\frac{\theta}{2}\right]\,\Pi_g{}^{R2}}{\sqrt{2}} + \frac{\text{Cos}\left[\frac{\theta}{2}\right]\,\sigma_{h,g}{}^{R2}}{\sqrt{2}}\right) \\
\alpha\,\text{Cos}\left[\frac{\theta}{2}\right]^7\,Z^{Q2}\,Z^{Q3}\,Z^{Q5}\,Z^{Q6}\,Z^{Q8}\,Z^{Q9}\left(-\frac{\text{Cos}\left[\frac{\theta}{2}\right]\,\Pi_h{}^{R2}}{\sqrt{2}} - \frac{\text{Cos}\left[\frac{\theta}{2}\right]\,\sigma_{g,h}{}^{R2}}{\sqrt{2}}\right) - \alpha\,\text{Cos}\left[\frac{\theta}{2}\right]\left(\frac{\text{Cos}\left[\frac{\theta}{2}\right]\,\Pi_h{}^{R2}}{\sqrt{2}} - \frac{\text{Cos}\left[\frac{\theta}{2}\right]\,\sigma_{g,h}{}^{R2}}{\sqrt{2}}\right) \\
\frac{\alpha\,\text{Cos}\left[\frac{\theta}{2}\right]\,\text{Sin}\left[\frac{\theta}{2}\right]}{\sqrt{2}} + \frac{\alpha\,\text{Cos}\left[\frac{\theta}{2}\right]^7\,\text{Sin}\left[\frac{\theta}{2}\right]\,Z^{Q2}\,Z^{Q3}\,Z^{Q5}\,Z^{Q6}\,Z^{Q8}\,Z^{Q9}}{\sqrt{2}} \\
-\alpha\,\text{Sin}\left[\frac{\theta}{2}\right] \\
\alpha\,\text{Cos}\left[\frac{\theta}{2}\right]^5\,\text{Sin}\left[\frac{\theta}{2}\right]\,Z^{Q2}\,Z^{Q5}\,Z^{Q6}\,Z^{Q8}\,Z^{Q9} \\
\alpha\,\text{Cos}\left[\frac{\theta}{2}\right]^4\,\text{Sin}\left[\frac{\theta}{2}\right]\,Z^{Q2}\,Z^{Q5}\,Z^{Q8}\,Z^{Q9} \\
\alpha\,\text{Cos}\left[\frac{\theta}{2}\right]^3\,\text{Sin}\left[\frac{\theta}{2}\right]\,Z^{Q2}\,Z^{Q5}\,Z^{Q8} \\
-\sqrt{2}\,\alpha\,\text{Cos}\left[\frac{\theta}{2}\right]^2\,\text{Sin}\left[\frac{\theta}{2}\right]\,Z^{Q2}\,Z^{Q5} \\
-\sqrt{2}\,\alpha\,\text{Cos}\left[\frac{\theta}{2}\right]\,\text{Sin}\left[\frac{\theta}{2}\right]\,Z^{Q2} \\
-\sqrt{2}\,\alpha\,\text{Sin}\left[\frac{\theta}{2}\right]
\end{pmatrix}$$

# Modelica netlist specification for lossy nine-qubit Z-probe and Z-feedback sub-circuits

- **Lossy Z-probe**

```
model BaconShorLossyZProbe
    Photonics.Components.SingleCavity  Q2(CavityType=Zprobe,  HilbertSpace=Q2)
    Photonics.Components.SingleCavity  Q5(CavityType=Zprobe,  HilbertSpace=Q5)
    Photonics.Components.SingleCavity  Q8(CavityType=Zprobe,  HilbertSpace=Q8)
    Photonics.Components.BeamSplitter  B1
    Photonics.Components.SingleCavity  Q7(CavityType=Zprobe,  HilbertSpace=Q7)
```

```
    Photonics.Components.SingleCavity Q4(CavityType=Zprobe, HilbertSpace=Q4)
    Photonics.Components.SingleCavity Q1(CavityType=Zprobe, HilbertSpace=Q1)
    Photonics.Components.SingleCavity Q9(CavityType=Zprobe, HilbertSpace=Q9)
    Photonics.Components.SingleCavity Q6(CavityType=Zprobe, HilbertSpace=Q6)
    Photonics.Components.SingleCavity Q3(CavityType=Zprobe, HilbertSpace=Q3)
    Photonics.Components.RelaySigma R1(HilbertSpace=R1)
    Photonics.Components.RelaySigma R2(HilbertSpace=R2)
    Photonics.Components.CoherentField W1(Amplitude=sqrt2alpha)
    Photonics.Components.CoherentField W2(Amplitude=alpha)
    Photonics.Components.CoherentField W3(Amplitude=alpha)
    Photonics.Components.BeamSplitter B2
    Photonics.Components.BeamSplitter B3
    Photonics.Components.Phase U
    Photonics.Components.Phase U1
    Photonics.Components.Phase U2
    Photonics.Components.Phase U3
    Photonics.Components.Phase U4
    Photonics.Components.Loss L1
    Photonics.Components.Loss L19
    Photonics.Components.Loss L3
    Photonics.Components.Loss L5
    Photonics.Components.Loss L6
    Photonics.Components.Loss L7
    Photonics.Components.Loss L8
    Photonics.Components.Loss L9
    Photonics.Components.Loss L10
    Photonics.Components.Loss L11
    Photonics.Components.Loss L12
    Photonics.Components.Loss L13
    Photonics.Components.Loss L14
    Photonics.Components.Loss L15
    Photonics.Components.Loss L16
    Photonics.Components.Loss L17
    Photonics.Components.Loss L18
equation
    connect(L9.output1,U1.input1)
    connect(U2.output1,B2.input2)
    connect(Q8.output1,B1.input1)
    connect(Q1.output1,L9.input1)
    connect(L13.output1,U2.input1)
    connect(W2.output1,L13.input1)
    connect(L16.output1,R1.input2)
    connect(L15.output1,R1.input1)
    connect(B2.output2,L16.input1)
    connect(B2.output1,L15.input1)
    connect(U1.output1,B2.input1)
    connect(L8.output1,Q1.input1)
    connect(L18.output1,R2.input2)
    connect(B3.output2,L18.input1)
    connect(L17.output1,R2.input1)
    connect(B3.output1,L17.input1)
```

```
    connect(U3.output1,B3.input2)
    connect(W3.output1,L14.input1)
    connect(L14.output1,U3.input1)
    connect(L12.output1,U4.input1)
    connect(Q3.output1,L12.input1)
    connect(Q6.output1,L11.input1)
    connect(L10.output1,Q6.input1)
    connect(Q9.output1,L10.input1)
    connect(L6.output1,Q9.input1)
    connect(B1.output2,L6.input1)
    connect(Q4.output1,L8.input1)
    connect(L7.output1,Q4.input1)
    connect(Q7.output1,L7.input1)
    connect(U.output1,Q7.input1)
    connect(L5.output1,U.input1)
    connect(B1.output1,L5.input1)
    connect(L3.output1,Q8.input1)
    connect(Q5.output1,L3.input1)
    connect(L19.output1,Q5.input1)
    connect(Q2.output1,L19.input1)
    connect(L1.output1,Q2.input1)
    connect(W1.output1,L1.input1)
    connect(L11.output1,Q3.input1)
    connect(U4.output1,B3.input1)
end BaconShorLossyZProbe
```

- **Lossy Z-feedback**

```
model BaconShorLossyZFeedback
    Photonics.Components.SingleCavity Q1(CavityType=Ramanh, HilbertSpace=Q1)
    Photonics.Components.SingleCavity Q2(CavityType=Ramanh, HilbertSpace=Q2)
    Photonics.Components.SingleCavity Q3(CavityType=Ramanh, HilbertSpace=Q3)
    Photonics.Components.CoherentField W1(Amplitude=betaOsqrt2)
    Photonics.Components.CoherentField W2(Amplitude=betaOsqrt2)
    Photonics.Components.SingleCavity R1(CavityType=Zprobe, HilbertSpace=R1)
    Photonics.Components.BeamSplitter B1
    Photonics.Components.BeamSplitter B2
    Photonics.Components.CoherentField W3(Amplitude=betaOsqrt2)
    Photonics.Components.CoherentField W4(Amplitude=betaOsqrt2)
    Photonics.Components.SingleCavity R2(CavityType=Zprobe, HilbertSpace=R2)
    Photonics.Components.BeamSplitter B3
    Photonics.Components.BeamSplitter B4
    Photonics.Components.SingleCavity q1(CavityType=Ramang, HilbertSpace=Q1)
    Photonics.Components.SingleCavity q2(CavityType=Ramang, HilbertSpace=Q2)
    Photonics.Components.SingleCavity q3(CavityType=Ramang, HilbertSpace=Q3)
    Photonics.Components.Phase U1
    Photonics.Components.Loss L1
    Photonics.Components.Loss L2
    Photonics.Components.Loss L3
    Photonics.Components.Loss L4
    Photonics.Components.Loss L5
    Photonics.Components.Loss L6
```

```
    Photonics.Components.Loss L7
    Photonics.Components.Loss L8
    Photonics.Components.Loss L9
    Photonics.Components.Loss L10
    Photonics.Components.Loss L11
    Photonics.Components.Loss L12
    Photonics.Components.Loss L13
    Photonics.Components.Loss L14
equation
    connect(L8.output1,B3.input2)
    connect(L6.output1,Q2.input1)
    connect(B2.output2,L6.input1)
    connect(L7.output1,Q1.input1)
    connect(B2.output1,L7.input1)
    connect(B1.output1,L4.input1)
    connect(L4.output1,U1.input1)
    connect(L5.output1,B2.input2)
    connect(B1.output2,L5.input1)
    connect(L2.output1,B1.input2)
    connect(W2.output1,L2.input1)
    connect(L3.output1,B1.input1)
    connect(R1.output1,L3.input1)
    connect(L1.output1,R1.input1)
    connect(W1.output1,L1.input1)
    connect(L11.output1,q1.input1)
    connect(B3.output1,L11.input1)
    connect(L13.output1,q3.input1)
    connect(B4.output2,L13.input1)
    connect(L12.output1,B4.input2)
    connect(B3.output2,L12.input1)
    connect(L14.output1,q2.input1)
    connect(B4.output1,L14.input1)
    connect(L9.output1,R2.input1)
    connect(W3.output1,L9.input1)
    connect(L10.output1,B3.input1)
    connect(R2.output1,L10.input1)
    connect(W4.output1,L8.input1)
    connect(U1.output1,Q3.input1)
end BaconShorLossyZFeedback
```
